# Supplementary material for: KoReA-SFL: Knowledge Replay-based Split Federated Learning Against Catastrophic Forgetting
Source: arXiv:2404.12846 source file (2024-04-19)
Supplement: Supplementary file 1 [file appendix.tex]

\clearpage
\appendix
\section{Convergence Analysis}
\label{sec:analysis}

% Inspired by the proof of the convergence of traditional one-to-multi FL approach~\cite{convergence,karimireddy2020scaffold}, we prove the convergence of our method as follows.

\subsubsection{Notations}
We assume that all clients adopt Stochastic Gradient Descent (SGD) as the optimizer.
Let $t$ be the current round of stochastic gradient descent
%of SGD iterations on the client, 
and 
$w^i_t=w^{c_i}_t\oplus w^{s_i}_t$ be the parameters of the $i^{th}$ complete middleware model that combines the client-side model $w^{c_i}_t$ and server-side model $w^{s_i}_t$. After one SGD iteration, we can get the parameters of the middleware model $v^i_{t+1}=v^{c_i}_{t+1}\oplus v^{s_i}_{t+1}$, where the $v^{c_i}_{t+1}$ and $v^{s_i}_{t+1}$ denote the client-side model and serve-side model respectively. 

Assume that in each SL round, each local model performs E rounds of SGD iterations, we have
\begin{equation}
\footnotesize
\begin{split}
w_{t+1}^i=\left\{
\begin{array}{rl}
v_{t+1}^i, &if (t + 1) \% E \neq 0 \\
\alpha v_{t+1}^i + (1-\alpha)\overline{v}_{t+1}, &if  (t + 1) \% E = 0\\
\end{array},
\right.  
\end{split}
\nonumber 
\end{equation}

where $\overline{v}_{t+1} = \frac{1}{N} \sum_{i=1}^{N} v_{t+1}^i$. 

In one SGD iteration, the update of the models follows the steps below:
\begin{enumerate}
    \item The client-side model $v^{c_i}_t$ perform forward propagation with a data batch $\xi_t^i$ and we can get the intermediate feature $y_c$
\begin{align}
    y_c = \nonumber w^{c_i}_{t}(\xi_t^i)\nonumber
\end{align}

    \item The server samples some features $y_h$ from assistant clients. After that, the server uses the feature $y_s=torch.cat(y_c,y_h)$ to perform forward propagation and update the server-side model using the following formula:
\begin{equation}
    v^{s_i}_{t+1}=w^{s_i}_t-\eta_t\nabla (\ell  (y)) \nonumber
\end{equation}
where $y$ denotes the output of the forward propagation $\ell$ denotes the loss function at the server side.

    \item After updating the server-side model, we update the client-side model using the following formula:
\begin{equation}
    v^{c_i}_{t+1}=v^{c_i}_{t}-\eta_t\nabla (\frac{\partial \ell(y)}{\partial f_c} ) \nonumber
\end{equation}
\end{enumerate}

To facilitate the prove, we define $g^i_t$ to denote the gradients of the model in the $i^{th}$ client after training with a data batch $\xi_t^i$:
\begin{equation}
\begin{split}
    g^i_t =\nabla f_i (w_t^i; \xi_t^i)=torch.cat(\nabla (\frac{\partial \ell(y)}{\partial f_c} ),\nabla (\ell  (y)) )
\end{split}
\nonumber 
\end{equation}
And we update the full middleware model $v_{t+1}^i$ by the following formula:
\begin{equation}
\footnotesize
\begin{split}
v_{t+1}^i = w_t^i - \eta_t \nabla f_i (w_t^i, \xi_t^i), 
\end{split}
\nonumber 
\end{equation}

Let $\overline{v}_t$ and $\overline{w}_t$ be the aggregated model of all middleware models, respectively. Since KoReA-SFL aggregates all the middleware models to gain the global model, we have
\begin{equation}
\footnotesize
\begin{split}
    \overline{v}_t = \frac{1}{N} \sum_{i=1}^{N} v_t^i, \ 
    \overline{w}_t = \frac{1}{N} \sum_{i=1}^{N} w_t^i.
\end{split}
\nonumber 
\end{equation}

%%%%%%%%%%%%%%%%%%%%%%%%%%%%%%%%%%%%%%%%%%%

\subsubsection{Proofs of Key Lemmas}
We analyze the convergence of KoReA-SFL based on three assumptions for the loss function of each client (i.e., $f_1, f_2, ...,$ or $f_N$), including $L$-smooth assumption (Assumption \ref{asm1}), $\mu$-convex assumption (Assumption \ref{asm2}), and variance/mean bound assumption for stochastic gradients (Assumption \ref{asm3}).

%where Assumptions \ref{asm1} and \ref{asm2} are standard \cite{convergence, stich2018local}, and Assumption \ref{asm3} has been made by the works in \cite{ zhang2012communication, stich2018local, convergence}.
% \newtheorem{assumption}{Assumption}
% \begin{assumption}\label{asm1}
% $f_i$ is $L$-smooth satisfying $f_i(w)\le f_i(w^\prime)+(w-w^\prime)^T\nabla f_i(w^\prime)+\frac{L}{2}||w-w^\prime||^2_2$, where $i \in\{ 1, 2, \cdots, N\}$.
% \end{assumption}
% %
% \begin{assumption}\label{asm2}
% $f_i$ is $\mu$-convex satisfying $f_i(w)\ge f_i(w^\prime)+(w-w^\prime)^T\nabla f_i(w^\prime)+\frac{\mu}{2}||w-w^\prime||^2_2$, where $i \in\{ 1, 2, \cdots, N\}$ and $\mu \geq 0$.
% \end{assumption}
% %
% \begin{assumption}\label{asm3}

% The variance of stochastic gradients is upper bounded by  $\sigma^2$ and the expectation of squared norm of stochastic gradients is upper bounded by  $G^2$, i.e.,  $\mathbb{E}||\nabla f_i (w;\xi) - \nabla f_i (w) ||^2 \leq \sigma^2$, $\mathbb{E}||\nabla f_i (w;\xi) ||^2 \leq G^2$, where $\xi$ is a  data batch of the $i^{th}$ client in the $t^{th}$ SFL round.
% \end{assumption}

Let $N$ be the number of clients that are participating in every SFL training round. Let $\{v^1_r,v^2_r,..,v^N_r\}$ be the set of uploaded local model parameters in the $(r-1)^{th}$ round, $\{w^1_r,w^2_r,..,w^N_r\}$ be the set of model parameters after model repository updating. Based on the implementation of our aggregation strategy, we have
% \begin{footnotesize}
\begin{equation}\label{eq:mr1}
\footnotesize
\begin{split}
w_{r}^i= \alpha v_{r}^i + (1-\alpha)\overline{v}_{r}.
\end{split}
\end{equation}
% \end{footnotesize}
According to the aggregation strategy of KoReA-SFL, we have
% \begin{footnotesize}
\begin{equation}\label{eq:mr2}
\footnotesize
\begin{split}
\sum_{i=1}^N w_{r}^i= \sum_{i=1}^N(\alpha v_{r}^i + (1-\alpha)\overline{v}_{r}) = \sum_{i=1}^N v_{r}^i
\end{split}
\end{equation}
% \end{footnotesize}
According to Equations~\ref{eq:mr1}-\ref{eq:mr2}, we can prove Lemma~\ref{eq:lemma1} as follows.
% \begin{lemma}\label{eq:lemma1} Let $w_{r}^i= \alpha v_{r}^i + (1-\alpha)\overline{v}_{r}$, $\alpha\in [0,1]$, and $\overline{w}_r = \sum_{i=1}^N w_{r}^i$. We have
% % \begin{footnotesize}
% \begin{equation}
% \footnotesize
% \begin{split}
% ||\overline{w}_r - w^\star||^2\leq\frac{1}{N}\sum_{i=1}^N||w_{r}^i-w^\star||^2\leq\frac{1}{N}\sum_{i=1}^N||v_{r}^i-w^\star||^2,
% \nonumber
% \end{split}
% \end{equation}
% % \end{footnotesize}
% where $w^\star$ is the optimal parameters for the global loss function $F(\cdot)$. In other words, $\forall w, F^\star\leq F(w)$, where $F^\star$ denotes $F(w^\star)$. 
% \end{lemma}

\begin{proof} %(Proof of Lemma~\ref{eq:lemma1})
According to equation \ref{eq:mr2}, we can derive the following inequality:
\begin{equation*}
\footnotesize
\begin{split}
\sum_{i=1}^N||w_{r}^i-w^\star||^2 & = \sum_{i=1}^N||\alpha v_{r}^i + (1-\alpha)\overline{v}_{r}-w^\star||^2\\
% & = (\alpha^2+(1-\alpha)^2)\sum_{k=1}^N ||v_r^k||^2 + 2\alpha(1-\alpha)\langle v_r^k,v_r^{k^\prime}\rangle + 2\sum_{k=1}^N\langle v_r^k, w^\star\rangle + ||w^\star||^2\\ 
% & = \sum_{i=1}^N[||v_r^i - w^\star||^2\\ &- \alpha(1-\alpha)(||v_r^i||^2 + 2\langle v_r^i,v_r^{i^\prime}\rangle + ||v_r^{i^\prime}||^2)]\\
& = \sum_{i=1}^N(||v_r^i - w^\star||^2 - \alpha(1-\alpha)||v_r^i - \overline{v}_{r}||^2)\\
&\leq \sum_{i=1}^N||v_r^i - w^\star||^2.
\end{split}
\end{equation*}

According to equation \ref{eq:mr2}, we have $\overline{v}_r= \overline{w}_r = \frac{1}{N}\sum_{i=1}^N w_r^i$. By using the AM–GM inequality, we can obtain:
\begin{small}
\begin{equation*}
||\overline{v}_r-w^\star||^2 \leq \frac{1}{N}\sum_{i=1}^N ||w_r^i-w^\star||^2.
\end{equation*}.
\end{small}
\end{proof}

To facilitate the convergence analysis of KoReA-SFL, we present Lemmas \ref{eq:lemma2}-\ref{eq:lemma3}.
\begin{lemma} \label{eq:lemma2} (Results of one  step SGD). If $\eta_t\leq \frac{1}{4L}$ holds, we have:
\begin{small}
\begin{equation*}
\footnotesize
\begin{split}
    \mathbb{E}||\overline{v}_{t+1} - w^\star||^2 \leq &\frac{1}{N}\sum_{i=1}^N(1-\mu\eta_t)||w^i_t -w^\star||^2 \\
    & + \frac{1}{N}\sum_{i=1}^N||w^i_t - w^i_{t_0}||^2 + 10\eta_t^2 L\Gamma.
\end{split}
. \nonumber
\end{equation*}
\end{small}
\end{lemma}

\begin{proof} %(Proof of Lemma~\ref{eq:lemma2})
By using the AM–GM inequality, it holds that:
\begin{equation*}
\footnotesize
\begin{split}
    ||\overline{v}_{t+1} - w^\star||^2 &
    \leq\frac{1}{N}\sum_{i=1}^N||v^i_{t+1} - w^\star||^2\\
     % & = \frac{1}{N}\sum_{i=1}^N||v^i_t - \eta_t g^i_t - w^\star||^2\\
     & = \frac{1}{N}\sum_{i=1}^N(||v^i_t -w^\star||^2 -2\eta_t \langle v^i_t-w^\star, g^i_t \rangle
     + \eta_t^2||g^i_t||^2).
\end{split}
\end{equation*}
Let $P_1 =  -2\eta_t\langle w^i_t-w^\star, g^i_t \rangle$ and $P_2=\eta_t^2\sum_{i=1}^N||g^i_t||^2$.
By using $\mu$-convex (Assumption \ref{asm2}), we have:
\begin{equation}\label{eq_b1}
\footnotesize
\begin{split}
P_1 \leq -2\eta_{t}(f_i (v^i_t)-f_i (w^\star))-\mu \eta_t ||w^i_t-w^\star||^2.
\end{split}
\end{equation}
By using $L$-smooth (Assumption \ref{asm1}), we obtain:
\begin{equation}\label{eq_b2}
\footnotesize
\begin{split}
P_2 \leq 2\eta_t^2 L (f_i(w_t^i)-f_i^\star).
\end{split}
\end{equation}
When $(t+1)\%E\neq 0$ and $v_t^i=w_t^i$ hold, according to Equations \ref{eq_b1}-\ref{eq_b2}, we have:
\begin{equation*}
\footnotesize
\begin{split}
    ||\overline{v}_{t+1} - w^\star||^2 
    \leq & \frac{1}{N}\sum_{i=1}^N [(1-\mu\eta_t)||v^i_t -w^\star||^2  -2\eta_{t}(f_i (w^i_t)-f_i (w^\star)) \\&+2\eta_t^2 L(f_i(w_t^i)-f_i^\star)].
\end{split}
\end{equation*}
    Let $P_3 = \frac{1}{N}\sum_{i=1}^N[-2\eta_{t}(f_i (w^i_t)-f_i (w^\star)) + 2\eta_t^2 L (f_i(w_t^i)-f_i^\star)]$. It holds that:
\begin{equation*}
\footnotesize
\begin{split}
    P_3 
    % &= \frac{-2\eta_{t}}{N}\sum_{i=1}^N(f_i (w^i_t)-f_i (w^\star)) + \frac{2\eta_t^2 L}{N}\sum_{i=1}^N(f_i(w_t^i)-f_i^\star)\\
    & = -\frac{2\eta_t(1-\eta_t L)}{N}\sum_{i=1}^N(f_i(w^i_t)-F^\star) + \frac{2\eta_t^2 L}{N}\sum_{i=1}^N(F^\star-f^\star_i).
\end{split}
\end{equation*}
Let $\Gamma=F^\star-\frac{1}{N}\sum_{i=1}^N f^\star_i$ and $\phi=2\eta_t(1-L\eta_t)$. We have:
\begin{equation*}
\footnotesize
\begin{split}
    P_3 = -\frac{\phi}{N}\sum_{i=1}^N(f_i(w^i_t)-F^\star) + 2\eta_t^2 L\Gamma.
\end{split}
\end{equation*}
Let $P_4=-\frac{1}{N}\sum_{i=1}^N(f_i(w^i_t)-F^\star)$, $t_0 \% E = 0$ and $t-t_0\leq E$. It holds that:
\begin{equation*}
\footnotesize
\begin{split}
    P_4 = -\frac{1}{N}\sum_{i=1}^N(f_i(w^i_t) - f_i(w^i_{t_0}) + f_i(w^i_{t_0}) -F^\star)
\end{split}.
\end{equation*}
Based on the Cauchy–Schwarz inequality, we can derive that:
\begin{equation}\label{eq_D}
\footnotesize
\begin{split}
    P_4 \leq & \frac{1}{2N}\sum_{i=1}^N(\eta_t ||\nabla f_i(w^i_{t_0})||^2 + \frac{1}{\eta_t}||w^i_t - w^i_{t_0}||^2)\\&  -\frac{1}{N}\sum_{i=1}^N(f_i(w^i_{t_0}) -F^\star)\\
     \leq& \frac{1}{2N}\sum_{i=1}^N \left[2\eta_t L(f_i(w^i_{t_0})-f_i^\star) + \frac{1}{\eta_t}||w^i_t - w^i_{t_0}||^2\right]\\& - \frac{1}{N}\sum_{i=1}^N(f_i(w^i_{t_0}) -F^\star).
\end{split}
\end{equation}

Note that, since $\eta\leq \frac{1}{4L}$, $\eta_t \leq \phi\leq 2\eta_t$ and $\eta_t L \leq \frac{1}{4}$, 
according to Equation \ref{eq_D}, we have:
\begin{equation*}
\footnotesize
\begin{split}
    P_3 &\leq\frac{\phi}{2N}\sum_{i=1}^N \left[2\eta_t L(f_i(w^i_{t_0})-f_i^\star) + \frac{1}{\eta_t}||w^i_t - w^i_{t_0}||^2\right]\\
    &- \frac{\phi}{N}\sum_{i=1}^N(f_i(w^i_{t_0}) -F^\star) + \eta_t^2 L\Gamma\\
    % & = \frac{\phi}{2\eta_t N}\sum_{i=1}^N||w^i_t - w^i_{t_0}||^2 + (\phi \eta_t L + 2\eta_t^2 L)\Gamma\\ & \qquad + \frac{\phi}{N}\sum_{i=1}^N(F^\star - f_i(w^i_{t_0}))\\
    & \leq \frac{\phi}{2\eta_t N}\sum_{i=1}^N||w^i_t - w^i_{t_0}||^2 + (\phi \eta_t L + 2\eta_t^2 L)\Gamma + \frac{\phi}{N}\sum_{i=1}^N(F^\star - f_i^\star)\\
    % &\leq \frac{\phi}{2\eta_t N}\sum_{i=1}^N||w^i_t - w^i_{t_0}||^2 + (\phi \eta_t L + \phi + 2\eta_t^2 L)\Gamma\\
    % &\leq  \frac{1}{N}\sum_{i=1}^N||w^i_t - w^i_{t_0}||^2 + (2\eta_t^2 L +2\eta_t) \Gamma\\
    &\leq  \frac{1}{N}\sum_{i=1}^N||w^i_t - w^i_{t_0}||^2 + 10\eta_t^2 L \Gamma.
\end{split}
\end{equation*}
\end{proof}

\begin{lemma} \label{eq:lemma3}
In KoReA-SFL, the server performs model aggregation after each E round of SGD to obtain the global model. For arbitrary $t$, there always exists $t_0 \leq t$ while $t_0$ is the last model aggregation closest to $t$.  As a result, $t - t_0 \leq E-1$ holds. Given the constraint on learning rate from \cite{convergence}, we know that $\eta_t \leq \eta_{t_0} \leq 2 \eta_t$. It follows that:
 % \begin{footnotesize}
\begin{equation*}
\footnotesize
\begin{split}
 \frac{1}{N} \sum_{i=1}^{N} ||w_t^i - {w}^i_{t_0}||^2 \leq 4\eta_t^2 (E - 1)^2 G^2.
\end{split}
\nonumber
\end{equation*}
% \end{footnotesize}
\end{lemma}

\begin{proof} 
Let $t_0\% E = 0$ and $t-t_0\leq E$. We have:
\begin{equation*}
\footnotesize
\begin{split}
\frac{1}{N} \sum_{i=1}^{N}||w_t^i - {w}^i_{t_0}||^2 = &\frac{1}{N} \sum_{i=1}^{N} \left|\left|\sum_{t=t_0}^{t_0 + E - 1} \eta_t \nabla f_{a_1}(w_t^{a_1};\xi_t^{a_1})\right|\right|^2   \\
% & \leq  (t - t_0) \sum_{t = t_0}^{t_0 + E - 1} \eta_t^2 G^2  \\  
& \leq  (E - 1) \sum_{t = t_0}^{t_0 + E - 1} \eta_t^2 G^2  \\
&\leq 4\eta_t^2 (E - 1)^2 G^2.
\end{split}
\nonumber
\end{equation*}
\end{proof}

Based on  Lemmas~\ref{eq:lemma1}-\ref{eq:lemma3}, we prove Theorem \ref{thm1} as follows.

\begin{thm}\label{thm1}
% Let Assumption \ref{asm1}, Assumption \ref{asm2}, Assumption \ref{asm3} hold. 
%After the recombination in each round, 
%we have
%Let $E$ be the number of SGD iterations of a round, and FedMR terminate afer $t=nE$ ($n\in N^+$) iterations, 
Assume that the server performs model aggregation after $E$ rounds of SGD,i.e., $E$ rounds of SGD are performed in each SFL round., and the whole training consists of $r$ SFL rounds. Let $t=r\times  E$ be the current number of SGD rounds, and $\eta_t=\frac{2} {\mu (t + \lambda)}$ be the learning rate. We have: 
% \begin{footnotesize}
% \vspace{-0.1in}
\begin{equation}
\label{eq:thm1}
\footnotesize
\begin{split}
\mathbb{E}[F(\overline{w}_t)] -F^\star \leq \frac{L}{2\mu(t+\lambda)}\left[\frac{4B}{\mu} + \frac{\mu(\lambda+1)}{2}\Delta_1\right]
    % \mathbb{E}||F(\overline{w}_t)|| - F^\star \leq \frac{L}{\mu(\gamma + t - 1)} (\frac{2 B}{\mu} + \frac{\mu \gamma}{2}\mathbb{E}||\overline{w}_1 - w^\star||^2)
\end{split},
\end{equation}
% \end{footnotesize}
where
\begin{small}
$
    B = 10 L \Gamma + 4(E - 1)^2 G^2.
     \nonumber
$
\end{small}
\end{thm}

\begin{proof} Let $\Delta_t = ||\overline{w}_t - w^\star||^2$ and $\Delta^{glb}_t = \frac{1}{N} \sum_{i=1}^{N}||w_t^i - {w}^\star||^2$.
According to Lemma \ref{eq:lemma1},  \ref{eq:lemma2}, and  \ref{eq:lemma3}, we have:
\begin{equation*}
\small
\begin{split}
    \Delta_{t+1} \leq \Delta^{glb}_{t+1} \leq (1-\mu\eta_t)\Delta^{glb}_{t} + \eta_t^2 B
\end{split}.\nonumber
\end{equation*}
When the step size becomes smaller, we have
 $\eta_t = \frac{\beta}{t + \lambda}$ for
 some $\beta > \frac{1}{\mu}$, $\lambda > 0$ such that $\eta_t \leq min\left\{\frac{1}{\mu},\frac{1}{4L}\right\}=\frac{1}{4L}$ and $\eta_t \leq 2\eta_{t+E}$.

Let $\theta = max\left\{\frac{\beta^2 B}{\mu\beta-1},(\lambda+1)\Delta_1\right\}$. We firstly prove  $\Delta_t\leq \frac{\theta}{t + \lambda}$ by induction.
When $t=1$,
\begin{equation}\label{eq:math_1}
\footnotesize
    \Delta_1 = \Delta^{glb}_1 = \frac{\lambda + 1}{\lambda + 1}\Delta_1 \leq \frac{\theta}{\lambda + 1}.
\end{equation}
Assuming
that $\Delta_t\leq\Delta^{glb}_t\leq \frac{\theta}{\lambda + 1}$, we have:
\begin{equation}\label{eq:math_t+1}
\footnotesize
\begin{split}
    \Delta_{t+1} & \leq \Delta^{glb}_{t+1}\\
    & \leq (1-\mu\eta_t)\Delta^{glb}_{t} + \eta_t^2 B\\
    % & = (1-\frac{\mu\beta}{t+\lambda})\frac{\theta}{t + \lambda} + \frac{\beta^2 B}{(t+\lambda)^2}\\
    & \leq \frac{t+\lambda - 1}{(t+\lambda)^2}\theta + \left[\frac{\beta^2 B}{(t+\lambda)^2} - \frac{\mu\beta -1}{(t+\lambda)^2}\theta\right]\\
    % & \leq \frac{t+\lambda - 1}{(t+\lambda)^2}\theta + \left[\frac{\beta^2 B}{(t+\lambda)^2} - \frac{\mu\beta -1}{(t+\lambda)^2}\frac{\beta^2 B}{\mu\beta-1}\right]\\
    & \leq \frac{\theta}{t+ 1 + \lambda}.
\end{split}
\end{equation}
According to Equations \ref{eq:math_1}-\ref{eq:math_t+1},
we have:
\begin{equation}\label{eq:math_proof}
\footnotesize
\begin{split}
{\small
     \Delta_t\leq \frac{\theta}{t + \lambda}}.
     \end{split}
\end{equation}
From Assumption \ref{asm1} and Equation~\ref{eq:math_proof}, we obtain:
\begin{equation}\label{t_1}
\footnotesize
\begin{split}
\mathbb{E}[f(\overline{w}_t)] -F^\star \leq \frac{L}{2}\Delta_{t}\leq \frac{\theta L}{2(t + \lambda)}.
\end{split}
\end{equation}
If we set $\beta =\frac{2}{\mu}$ and $\lambda=max\{\frac{10L}{\mu},E\}-1$, we have $\eta_t=\frac{2}{\mu(t + \lambda)}$ and $\eta_t \leq 2\eta_{t+E}$ for $t\ge 1$. Then, it holds that:
\begin{equation}\label{t_2}
\footnotesize
\begin{split}
\theta & =max\left\{\frac{\beta^2 B}{\mu\beta-1},(\lambda+1)\Delta_1\right\}\\
     & \leq \frac{\beta^2 B}{\mu\beta-1} +(\lambda+1)\Delta_1 \\
     & \leq \frac{4B}{\mu^2} + (\lambda+1)\Delta_1.
\end{split}
\end{equation}
Based on Equations \ref{t_1}-\ref{t_2}, we have:
\begin{equation*}
\footnotesize
\begin{split}
\mathbb{E}[F(\overline{w}_t)] -F^\star & \leq \frac{L}{2(t+\lambda)}\left[\frac{4B}{\mu^2} + (\lambda+1)\Delta_1\right]\\
& = \frac{L}{2\mu(t+\lambda)}\left[\frac{4B}{\mu} + \frac{\mu(\lambda+1)}{2}\Delta_1\right].
\end{split}
\end{equation*}
\end{proof}

From Theorem \ref{thm1}, we can observe that as the SGD round $t$ increases, the difference between the current loss $F(\overline{w}_t)$ and the optimal loss $F^\star$ will decrease and approach 0, indicating that KoReA-SFL will eventually converge.
% Theorem \ref{thm1} indicates that the difference between the current loss $F(\overline{w}_t)$ and the optimal loss $F^\star$ is inversely related to $t$. From Theorem \ref{thm1}, we observe that
% as the value of $t$ increases, the right side of Equation~\ref{eq:thm1} in Theorem~\ref{thm1} will approach 0, indicating that KoReA-SFL will eventually converge.
% In addition, we can also find that the convergence rate of KoReA-SFL is similar to that of FedAvg, which has been analyzed in \cite{convergence}. 
